# Supplementary material for: AgentBoard: An Analytical Evaluation Board of Multi-turn LLM Agents
Source: arXiv:2401.13178 source file (2024-12-23)
Supplement: Supplementary file 1 [file check.tex]

\section{Annotation of sub-goals}
We develop multiple methods for annotating sub-goals, broadly divided into: (1) observation-based, and (2) attribute-matching methods (Webshop and Webarena). For observation-based tasks, we annotate $N$ necessary observations to accomplish a goal, where the obtained reward score is the ratio of completed sub-goals to $N$. For tasks in the web category, we directly use of the matching score.
