# Supplementary material for: AgentBoard: An Analytical Evaluation Board of Multi-turn LLM Agents
Source: arXiv:2401.13178 source file (2024-12-23)
Supplement: Supplementary file 2 [file diificulty_level.tex]

\section{Difficulty Level Annotation\label{sec:difficulty_level_annotation}}

We annotate the level of the difficulties of different environment according to the number of subgoals.
