# Supplementary material for: AgentBoard: An Analytical Evaluation Board of Multi-turn LLM Agents
Source: arXiv:2401.13178 source file (2024-12-23)
Supplement: Supplementary file 3 [file reward_step_score.tex]

\section{Reward-step Score}

\begin{figure}
    \vspace{-0.3cm}
    \centering
    \includegraphics[width=\textwidth]{figures/reward_vs_steps.pdf}
    \caption{Reward-step scores of the tasks of \junlei{the reward-step score of other tasks should be placed here}}
    \label{fig:reward_vs_steps_others}
\end{figure}
